# Supplementary material for: Personalized Decision Making for Biopsies in Prostate Cancer Active Surveillance Programs
Source: arXiv:1907.05621 source file (2019-07-12)
Supplement: Supplementary file 1 [file Appendix_online_supp.pdf]

# Supplementary Materials for "Personalized Decision Making for Biopsies in Prostate Cancer Active Surveillance Programs"

Anirudh Tomer[1,*], Dimitris Rizopoulos[1], Daan Nieboer[2], Frank-Jan Drost[3], Monique J. Roobol[3], and Ewout W. Steyerberg[2,4]

[1]Department of Biostatistics, Erasmus University Medical Center, the Netherlands
[2]Department of Public Health, Erasmus University Medical Center, the Netherlands
[3]Department of Urology, Erasmus University Medical Center, the Netherlands
[4]Department of Biomedical Data Sciences, Leiden University Medical Center, the Netherlands
[*]*email*: a.tomer@erasmusmc.nl

## Appendix A  A Bivariate Joint Model for the Longitudinal PSA, and DRE Measurements, and Time to Cancer Progression

In this appendix section, we first provide an introduction to the world's largest active surveillance (AS) program called Prostate Cancer Research International Active Surveillance, abbreviated as PRIAS (Bokhorst et al., 2016), that we use to develop our methodology. We then present an introduction to the joint models for time-to-event and bivariate longitudinal data (Rizopoulos, 2012; Tsiatis and Davidian, 2004), that we fit to the PRIAS dataset. Lastly, we present the parameter estimation for our model using the Bayesian approach.

### Appendix A.1  PRIAS Dataset

To develop our methodology we use the data of prostate cancer patients (see Table 1) from the world's largest AS study called PRIAS (Bokhorst et al., 2016). More than 100 medical centers from 17 countries worldwide contribute to the collection of data, utilizing a common study protocol and a web-based tool, both available at `www.prias-project.org`. We use data collected over a period of ten years, between December 2006 (beginning of PRIAS study) and December 2016. The primary event of interest is cancer progression detected upon a positive biopsy. Biopsies are scheduled at the following fixed follow-up times (measured since inclusion in AS): year 1, 4, 7, and 10, and every 5 years thereafter. An annual schedule of biopsies is prescribed to those patients who have a PSA (prostate-specific antigen) doubling time between 0 and 10 years. The PSA doubling time at any point during follow-up is measured as the inverse of the slope of the regression line through the base two logarithm of the observed PSA values. The time of cancer progression is

Table 1: **Summary statistics for the PRIAS dataset**. The primary event of interest is cancer progression. A DRE measurement equal to T1c (Schröder et al., 1992) indicates a clinically inapparent tumor which is not palpable or visible by imaging, while tumors with DRE > T1c are palpable. The abbreviation IQR means interquartile range.

| Data | Value |
|---|---|
| Total patients | 5270 |
| Cancer progression (primary event) | 866 |
| Loss to follow-up (anxiety or unknown) | 685 |
| Patient removal on the basis of PSA and DRE | 464 |
| Death (unrelated to prostate cancer) | 61 |
| Death (related to prostate cancer) | 2 |
| Median Age (years) | 70 (IQR: 65–75) |
| Total PSA measurements | 46015 |
| Median number of PSA measurements per patient | 7 (IQR: 7–12) |
| Median PSA value (ng/mL) | 5.6 (IQR: 4.0–7.5) |
| Total DRE measurements | 25606 |
| Median number of DRE measurements per patient | 4 (IQR: 3–7) |
| DRE = T1c (%) | 23538/25606 (92%) |

interval censored because biopsies are scheduled periodically. There are three types of competing events, namely death, removal of patients from AS on the basis of their observed DRE and PSA measurements, and loss to follow-up. We assume these three types of events to be censored observations (see Appendix A.5 for details). However, our model allows removal of patients to depend on observed longitudinal data and baseline covariates of the patient. Under the aforementioned assumption of censoring, Figure 1 shows the cumulative risk of cancer progression over the study follow-up period.

For all patients, PSA measurements (ng/mL) are scheduled every 3 months for the first 2 years and every 6 months thereafter. The DRE measurements are scheduled every 6 months. We use the DRE measurements as DRE = T1c versus DRE > T1c. A DRE measurement equal to T1c (Schröder et al., 1992) indicates a clinically inapparent tumor which is not palpable or visible by imaging, while tumors with DRE > T1c are palpable.

**Data Accessibility:** The PRIAS database is not openly accessible. However, access to the database can be requested on the basis of a study proposal approved by the PRIAS steering committee. The website of the PRIAS program is `www.prias-project.org`.

## Appendix A.2 Model Definition

Let $T_i^*$ denote the true cancer progression time of the $i$-th patient included in PRIAS. Since biopsies are conducted periodically, $T_i^*$ is observed with interval censoring $l_i < T_i^* \leq r_i$. When progression is observed for the patient at his latest biopsy time $r_i$, then $l_i$ denotes the time of the second latest biopsy. Otherwise, $l_i$ denotes the time of the latest biopsy and $r_i = \infty$. Let $\boldsymbol{y}_{di}$ and $\boldsymbol{y}_{pi}$ denote his observed DRE and PSA longitudinal measurements, respectively. The observed data of all $n$ patients is denoted by $\mathcal{D}_n = \{l_i, r_i, \boldsymbol{y}_{di}, \boldsymbol{y}_{pi}; i = 1, \ldots, n\}$.

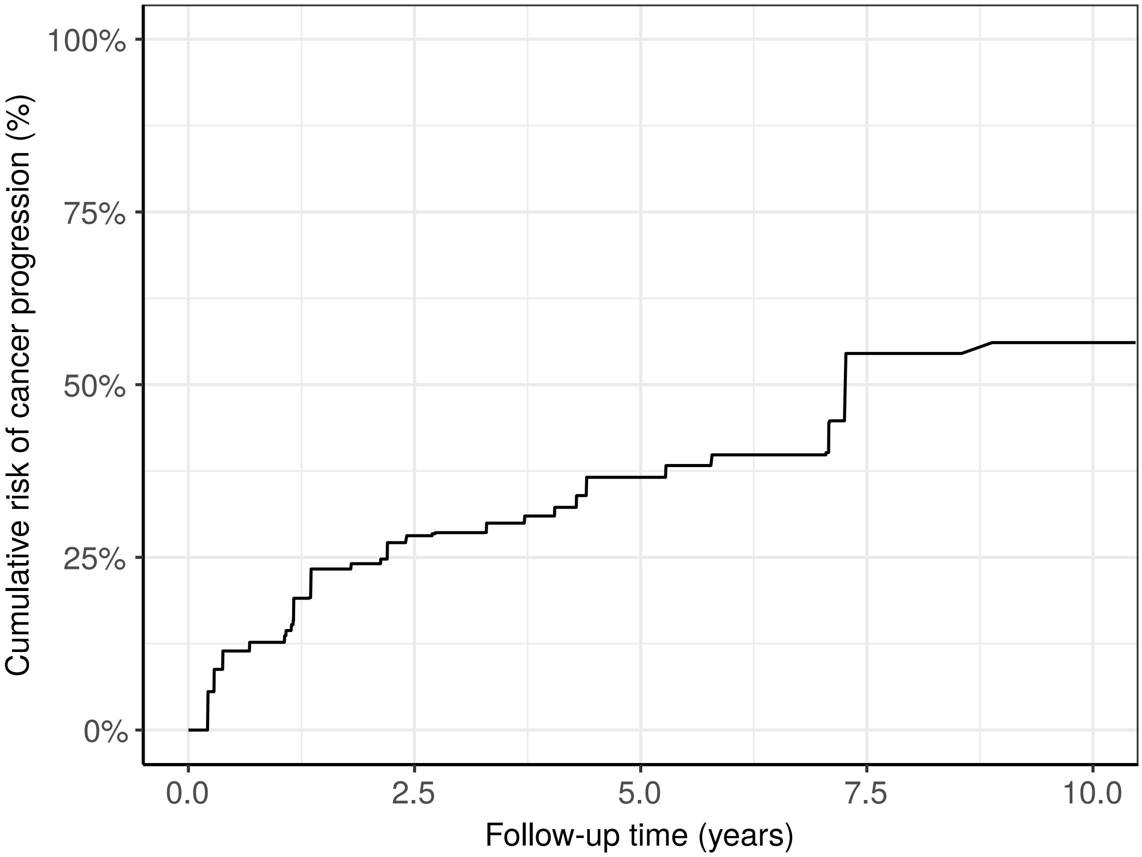


Figure 1: **Estimated cumulative risk of cancer progression in AS** for patients in the Prostate Cancer Research International Active Surveillance (PRIAS) dataset. Nearly 50% patients (*slow progressing*) do not progress in the ten year follow-up period. Cumulative risk is estimated using nonparametric maximum likelihood estimation (Turnbull, 1976), to account for interval censored cancer progression times observed in the PRIAS dataset. Censoring includes death, removal from AS on the basis of observed longitudinal data, and patient dropout.

In our joint model, the patient-specific DRE and PSA measurements over time are modeled using a bivariate generalized linear mixed effects sub-model. The sub-model for DRE is given by (see Panel A, Figure 2):

$$\begin{aligned}\text{logit}\big[\Pr\{y_{di}(t) > \text{T1c}\}\big] &= \beta_{0d} + b_{0di} + (\beta_{1d} + b_{1di})t \\ &+ \beta_{2d}(\text{Age}_i - 70) + \beta_{3d}(\text{Age}_i - 70)^2 \end{aligned} \tag{1}$$

where, $t$ denotes the follow-up visit time, and $\text{Age}_i$ is the age of the $i$-th patient at the time of inclusion in AS. The fixed effect parameters are denoted by $\{\beta_{0d}, \ldots, \beta_{3d}\}$, and $\{b_{0di}, b_{1di}\}$ are the patient specific random effects. With this definition, we assume that the patient-specific log odds of obtaining a DRE measurement larger than T1c remain linear over time.

The mixed effects sub-model for PSA is given by (see Panel B, Figure 2):

$$\begin{aligned}\log_2\big\{y_{pi}(t) + 1\big\} &= m_{pi}(t) + \varepsilon_{pi}(t), \\ m_{pi}(t) &= \beta_{0p} + b_{0pi} + \sum_{k=1}^{4}(\beta_{kp} + b_{kpi})B_k(t, \mathcal{K}) \\ &+ \beta_{5p}(\text{Age}_i - 70) + \beta_{6p}(\text{Age}_i - 70)^2, \end{aligned} \tag{2}$$

where, $m_{pi}(t)$ denotes the underlying measurement error free value of $\log_2(\text{PSA} + 1)$

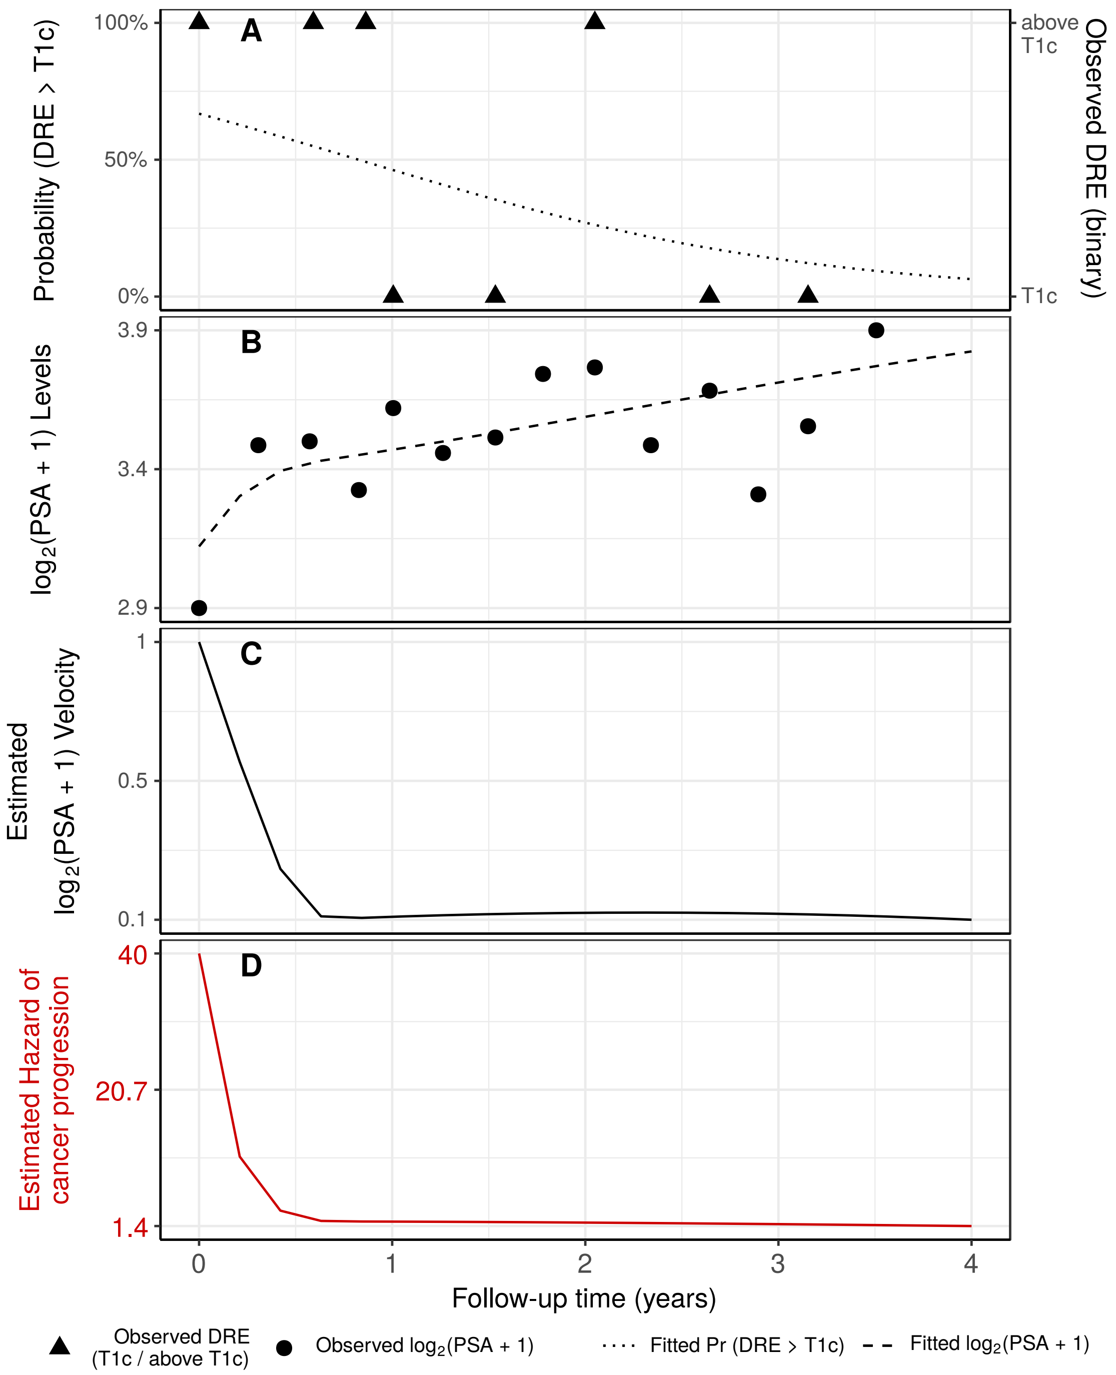


Figure 2: **Illustration of the joint model fitted to the PRIAS dataset**. **Panel A:** shows the observed DRE measurements and the fitted probability of obtaining DRE > T1c (Equation 1) for . **Panel B:** shows the observed and fitted $\log_2(\text{PSA} + 1)$ measurements (Equation 2). **Panel C:** shows the estimated $\log_2(\text{PSA}+1)$ velocity (velocity cannot be observed directly) over time. The hazard function (Equation 3) shown in **Panel D**, depends on the fitted log odds of having a DRE > T1c, and the fitted $\log_2(\text{PSA} + 1)$ value and velocity.

transformed (Lin et al., 2000; Pearson et al., 1994) measurements at time $t$. We model it non-linearly over time using B-splines (De Boor, 1978). To this end, our B-spline basis function $B_k(t, \mathcal{K})$ has 3 internal knots at $\mathcal{K} = \{0.1, 0.7, 4\}$ years, and boundary knots at 0 and 5.42 years (95-th percentile of the observed follow-up times). The fixed effect parameters are denoted by $\{\beta_{0p}, \ldots, \beta_{6p}\}$, and $\{b_{0pi}, \ldots, b_{4pi}\}$ are the

patient specific random effects. The error $\varepsilon_{pi}(t)$ is assumed to be t-distributed with three degrees of freedom (see Appendix B.1) and scale $\sigma$, and is independent of the random effects.

To account for the correlation between the DRE and PSA measurements of a patient, we link their corresponding random effects. More specifically, the complete vector of random effects $\boldsymbol{b}_i = (b_{0di}, b_{1di}, b_{0pi}, \ldots, b_{4pi})^T$ is assumed to follow a multivariate normal distribution with mean zero and variance-covariance matrix $\boldsymbol{D}$.

To model the impact of DRE and PSA measurements on the risk of cancer progression, our joint model uses a relative risk sub-model. More specifically, the hazard of cancer progression $h_i(t)$ at a time $t$ is given by (see Panel D, Figure 2):

$$\begin{aligned} h_i(t) = h_0(t) \exp\Big(&\gamma_1(\text{Age}_i - 70) + \gamma_2(\text{Age}_i - 70)^2 \\ &+ \alpha_{1d}\text{logit}\big[\Pr\{y_{di}(t) > \text{T1c}\}\big] + \alpha_{1p} m_{pi}(t) + \alpha_{2p}\frac{\partial m_{pi}(t)}{\partial t}\Big), \end{aligned} \tag{3}$$

where, $\gamma_1, \gamma_2$ are the parameters for the effect of age. The parameter $\alpha_{1d}$ models the impact of log odds of obtaining a DRE $>$ T1c on the hazard of cancer progression. The impact of PSA on the hazard of cancer progression is modeled in two ways: a) the impact of the error free underlying PSA value $m_{pi}(t)$ (see Panel B, Figure 2), and b) the impact of the underlying PSA velocity $\partial m_{pi}(t)/\partial t$ (see Panel C, Figure 2). The corresponding parameters are $\alpha_{1p}$ and $\alpha_{2p}$, respectively. Lastly, $h_0(t)$ is the baseline hazard at time t, and is modeled flexibly using P-splines (Eilers and Marx, 1996). More specifically:

$$\log h_0(t) = \gamma_{h_0,0} + \sum_{q=1}^{Q} \gamma_{h_0,q} B_q(t, \boldsymbol{v}),$$

where $B_q(t, \boldsymbol{v})$ denotes the $q$-th basis function of a B-spline with knots $\boldsymbol{v} = v_1, \ldots, v_Q$ and vector of spline coefficients $\gamma_{h_0}$. To avoid choosing the number and position of knots in the spline, a relatively high number of knots (e.g., 15 to 20) are chosen and the corresponding B-spline regression coefficients $\gamma_{h_0}$ are penalized using a differences penalty (Eilers and Marx, 1996). An example fitted hazard is shown in panel D of Figure 2.

## Appendix A.3 Parameter Estimation

We estimate the parameters of the joint model using Markov chain Monte Carlo (MCMC) methods under the Bayesian framework. Let $\boldsymbol{\theta}$ denote the vector of all of the parameters of the joint model. The joint model postulates that given the random effects, the time to cancer progression, and the DRE and PSA measurements taken over time are all mutually independent. Under this assumption the posterior distribution of the parameters is given by:

$$\begin{aligned} p(\boldsymbol{\theta}, \boldsymbol{b} \mid \mathcal{D}_n) &\propto \prod_{i=1}^{n} p(l_i, r_i, \boldsymbol{y}_{di}, \boldsymbol{y}_{pi}, \mid \boldsymbol{b}_i, \boldsymbol{\theta}) p(\boldsymbol{b}_i \mid \boldsymbol{\theta}) p(\boldsymbol{\theta}) \\ &\propto \prod_{i=1}^{n} p(l_i, r_i \mid \boldsymbol{b}_i, \boldsymbol{\theta}) p(\boldsymbol{y}_{di} \mid \boldsymbol{b}_i, \boldsymbol{\theta}) p(\boldsymbol{y}_{pi} \mid \boldsymbol{b}_i, \boldsymbol{\theta}) p(\boldsymbol{b}_i \mid \boldsymbol{\theta}) p(\boldsymbol{\theta}), \\ p(\boldsymbol{b}_i \mid \boldsymbol{\theta}) &= \frac{1}{\sqrt{(2\pi)^q \det(\boldsymbol{D})}} \exp(\boldsymbol{b}_i^T \boldsymbol{D}^{-1} \boldsymbol{b}_i), \end{aligned}$$

where, the likelihood contribution of the DRE outcome, conditional on the random effects is:

$$p(\boldsymbol{y}_{di} \mid \boldsymbol{b}_i, \boldsymbol{\theta}) = \prod_{k=1}^{n_{di}} \frac{\exp\Big[-\text{logit}\big\{\Pr(y_{dik} > \text{T1c})\big\} I(y_{dik} = \text{T1c})\Big]}{1 + \exp\Big[-\text{logit}\big\{\Pr(y_{dik} > \text{T1c})\big\}\Big]},$$

where $I(\cdot)$ is an indicator function which takes the value 1 if the $k$-th repeated DRE measurement $y_{dik} = \text{T1c}$, and takes the value 0 otherwise. The likelihood contribution of the PSA outcome, conditional on the random effects is:

$$p(\boldsymbol{y}_{pi} \mid \boldsymbol{b}_i, \boldsymbol{\theta}) = \frac{1}{\big(\sqrt{2\pi\sigma^2}\big)^{n_{pi}}} \exp\bigg(-\frac{\lVert \boldsymbol{y}_{pi} - \boldsymbol{m}_{pi} \rVert^2}{\sigma^2}\bigg),$$

The likelihood contribution of the time to cancer progression outcome is given by:

$$p(l_i, r_i \mid \boldsymbol{b}_i, \boldsymbol{\theta}) = \exp\Big\{-\int_0^{l_i} h_i(s)\mathrm{d}s\Big\} - \exp\Big\{-\int_0^{r_i} h_i(s)\mathrm{d}s\Big\}. \tag{4}$$

The integral in (4) does not have a closed-form solution, and therefore we use a 15-point Gauss-Kronrod quadrature rule to approximate it.

We use independent normal priors with zero mean and variance 100 for the fixed effects $\{\beta_{0d}, \ldots, \beta_{3d}, \beta_{0p}, \ldots, \beta_{6p}\}$, and inverse Gamma prior with shape and rate both equal to 0.01 for the parameter $\sigma^2$. For the variance-covariance matrix $\boldsymbol{D}$ of the random effects we take inverse Wishart prior with an identity scale matrix and degrees of freedom equal to 7 (number of random effects). For the relative risk model's parameters $\{\gamma_1, \gamma_2\}$ and the association parameters $\{\alpha_{1d}, \alpha_{1p}, \alpha_{2p}\}$, we use independent normal priors with zero mean and variance 100.

## Appendix A.4 Personalized Posterior Predictive Distribution of Time of Cancer Progression

Let us assume a new patient $j$, for whom we need to make a personalized biopsy decision. Let his current follow-up visit time be $s$, latest time of biopsy be $t \leq s$, observed vectors of DRE and PSA measurements be $\mathcal{Y}_{dj}(s)$ and $\mathcal{Y}_{pj}(s)$, respectively. The combined information from the observed data is given by the following posterior predictive distribution $g(T_j^*)$ of his time of cancer progression $T_j^*$:

$$\begin{aligned} g(T_j^*) &= p\big\{T_j^* \mid T_j^* > t, \mathcal{Y}_{dj}(s), \mathcal{Y}_{pj}(s), \mathcal{D}_n\big\} \\ &= \int\int p\big(T_j^* \mid T_j^* > t, \boldsymbol{b}_j, \boldsymbol{\theta}\big) \\ &\quad \times p\big\{\boldsymbol{b}_j \mid T_j^* > t, \mathcal{Y}_{dj}(s), \mathcal{Y}_{pj}(s), \boldsymbol{\theta}\big\} p\big(\boldsymbol{\theta} \mid \mathcal{D}_n\big) \mathrm{d}\boldsymbol{b}_j \mathrm{d}\boldsymbol{\theta}. \end{aligned}$$

The distribution $g(T_j^*)$ depends on observed data of the patient $\mathcal{Y}_{dj}(s)$ and $\mathcal{Y}_{pj}(s)$, as well information from the PRIAS dataset $\mathcal{D}_n$ via the posterior distribution of random effects $\boldsymbol{b}_j$ and posterior distribution of the vector of all parameters $\boldsymbol{\theta}$, respectively.

The distribution can be estimated as detailed in Rizopoulos, Molenberghs, and Lesaffre, (2017). However, majority of the prostate cancer patients do not progress in the ten year follow-up period of PRIAS (see Figure 1). Consequently, the personalized density function of cancer progression $g(T_j^*)$ can only be estimated for time points falling within the ten year follow-up.

## Appendix A.5 PSA Dependent Biopsy Schedule of PRIAS, and Competing Risks

**PSA dependent interval censored time of cancer progression:** The true time of cancer progression $T_i^*$ is not known for any of the patients in PRIAS. In order to detect cancer progression, PRIAS uses a fixed schedule of biopsies wherein biopsies are conducted at year one, year four, year seven and year ten of follow-up, and every five years thereafter. However, PRIAS switches to a more frequent annual biopsy schedule for faster-progressing patients. These are patients with PSA doubling time (PSA-DT) between 0 and 10 years, which is measured as the inverse of the slope of the regression line through the base two logarithm of PSA values. Thus, the interval $l_i < T_i^* \leq r_i$ in which cancer progression is detected depends on the observed PSA values.

**Competing events:** The primary event of interest in this paper is cancer progression observed via a positive biopsy. There are three types of competing events, namely death of 63 patients, of which 61 died from non prostate cancer related reasons; removal of 464 patients from AS on the basis of their observed DRE and PSA measurements; and loss to follow-up of 685 patients because of patient anxiety or unknown reasons. Death from non cancer related reasons impedes occurrence of cancer progression, and is indeed a competing event.

The number of patients obtaining the event death is small compared to the number of patients who obtain the primary event cancer progression. Hence in this paper considering death as non-informative censoring may be viable. We also consider loss to follow-up as non-informative censoring, which may not always be true. This is especially the case when the reason of loss to follow-up is unknown. However, when the reason of loss to follow-up is patient anxiety, it is often on the basis of their observed results. Given the large number of loss to follow-up patients, considering these patients as censored is a limitation of our work. However, the problem of unknown reason of dropout is not specific to only our model. For the remaining patients who are removed from AS on the basis their observed longitudinal data, the removal does not impede occurrence of cancer progression. In the next paragraph we show that the removal of these patients is non-informative about the parameters of the model for the true time of cancer progression.

Given the aforementioned issues of PSA dependent interval censoring and removal of patients on the basis of their observed longitudinal data is natural to question in this scenario if the parameters of the joint model are affected by these two. However, because the parameters of the joint model are estimated using a full likelihood approach (Tsiatis and Davidian, 2004), the joint model allows the schedule of biopsies, as well as censoring to depend upon the observed DRE and PSA measurements (e.g., via PSA-DT), under the condition that the model is correctly specified. To show this, consider the following full general specification of the joint model that we use. Let $\boldsymbol{y}_{di}, \boldsymbol{y}_{pi}$ denote the observed DRE and PSA measurements for the $i$-th patient, and $l_i, r_i$ denote the two time points of the interval in which GR occurs for the $i$-th patient. In addition let $T_i^S$ and $\mathcal{V}_{di}, \mathcal{V}_{pi}$ denote the schedule of biopsies, and the schedule of DRE and PSA measurements, respectively. Let $G_i^*$ denote the time of removal from AS without observing cancer progression. Under the assumption that $T_i^S, G_i^*, \mathcal{V}_{di}, \mathcal{V}_{pi}$ may depend upon only the observed data $\boldsymbol{y}_{di}, \boldsymbol{y}_{pi}$,

the joint likelihood of the various processes is given by:

$$\begin{aligned} p(\boldsymbol{y}_{di}, \boldsymbol{y}_{pi}, l_i, r_i, T_i^S, G_i^*, \mathcal{V}_{di}, \mathcal{V}_{pi} \mid \boldsymbol{\theta}, \boldsymbol{\psi}) = {} & p(\boldsymbol{y}_{di}, \boldsymbol{y}_{pi}, l_i, r_i \mid \boldsymbol{\theta}) \\ & \times p(T_i^S, G_i^*, \mathcal{V}_{di}, \mathcal{V}_{pi} \mid \boldsymbol{y}_{di}, \boldsymbol{y}_{pi}, \boldsymbol{\psi}). \end{aligned}$$

From this decomposition we can see that even if the processes $T_i^S, G_i^*, \mathcal{V}_{di}, \mathcal{V}_{pi}$ may be determined from $\boldsymbol{y}_{di}, \boldsymbol{y}_{pi}$, if we are interested in the parameters $\boldsymbol{\theta}$ of the joint distribution of longitudinal and event outcomes, we can maximize the likelihood based on the first term and ignore the second term. In other words, the second term will not carry information for $\boldsymbol{\theta}$. Lastly, since we use a full likelihood approach with an interval censoring specification, the estimates that we obtain are consistent and asymptotically unbiased (Gentleman and Geyer, 1994), despite the interval censoring observed.

# Appendix B Parameter Estimates from the Joint Model Fitted to the PRIAS Dataset

We fit a joint model to the PRIAS dataset using the R package **JMbayes** (Rizopoulos, 2016). The corresponding posterior parameter estimates are shown in Table 3 (longitudinal sub-model for DRE outcome), Table 4 (longitudinal sub-model for PSA outcome) and Table 5 (relative risk sub-model). The parameter estimates for the variance-covariance matrix $\boldsymbol{D}$ from the longitudinal sub-model are shown in the following Table 2:

Table 2: Estimated variance-covariance matrix $\boldsymbol{D}$ of the random effects $\boldsymbol{b} = (b_{0d}, b_{1d}, b_{0p}, b_{1p}, b_{2p}, b_{3p}, b_{4p})$ (see Appendix A.2) from the joint model fitted to the PRIAS dataset. The variances of the random effects are highlighted along the diagonal of the variance-covariance matrix.

| Random Effects | $b_{0d}$ | $b_{1d}$ | $b_{0p}$ | $b_{1p}$ | $b_{2p}$ | $b_{3p}$ | $b_{4p}$ |
|---|---|---|---|---|---|---|---|
| $b_{0d}$ | 7.55 | -0.56 | -0.18 | 0.08 | 0.084 | 0.003 | -0.019 |
| $b_{1d}$ | -0.564 | 1.379 | 0.081 | 0.119 | 0.165 | 0.266 | 0.219 |
| $b_{0p}$ | -0.182 | 0.081 | 0.208 | 0.031 | 0.034 | 0.068 | 0.014 |
| $b_{1p}$ | 0.075 | 0.119 | 0.031 | 0.224 | 0.109 | 0.158 | 0.088 |
| $b_{2p}$ | 0.084 | 0.165 | 0.034 | 0.109 | 0.293 | 0.324 | 0.238 |
| $b_{3p}$ | 0.003 | 0.266 | 0.068 | 0.158 | 0.324 | 0.480 | 0.312 |
| $b_{4p}$ | -0.019 | 0.219 | 0.014 | 0.088 | 0.238 | 0.312 | 0.290 |

For the DRE mixed effects sub-model (see Equation 1) parameter estimates, in Table 3 we can see that the age of the patient trivially affects the baseline log odds of obtaining a DRE measurement larger than T1c. In Figure 3 we present the marginal evolution of log odds of obtaining a DRE larger than T1c, and the corresponding marginal probability, over a period of 10 years for a hypothetical AS patient who is included in AS at the age of 70 years. In addition, we present plots of observed DRE versus fitted probabilities of obtaining a DRE measurement larger than T1c, for nine randomly selected patients in Figure 4.

Table 3: Estimated mean and 95% credible interval for the parameters of the longitudinal sub-model (see Equation 1) for the DRE outcome.

| Variable | Mean | Std. Dev | 2.5% | 97.5% | P |
|---|---|---|---|---|---|
| (Intercept) | -4.017 | 0.136 | -4.270 | -3.763 | <0.001 |
| (Age − 70) | 0.058 | 0.009 | 0.041 | 0.075 | <0.001 |
| $(\text{Age} - 70)^2$ | -0.001 | 0.001 | -0.003 | 0.000 | 0.076 |
| visitTimeYears | -0.604 | 0.095 | -0.794 | -0.437 | <0.001 |

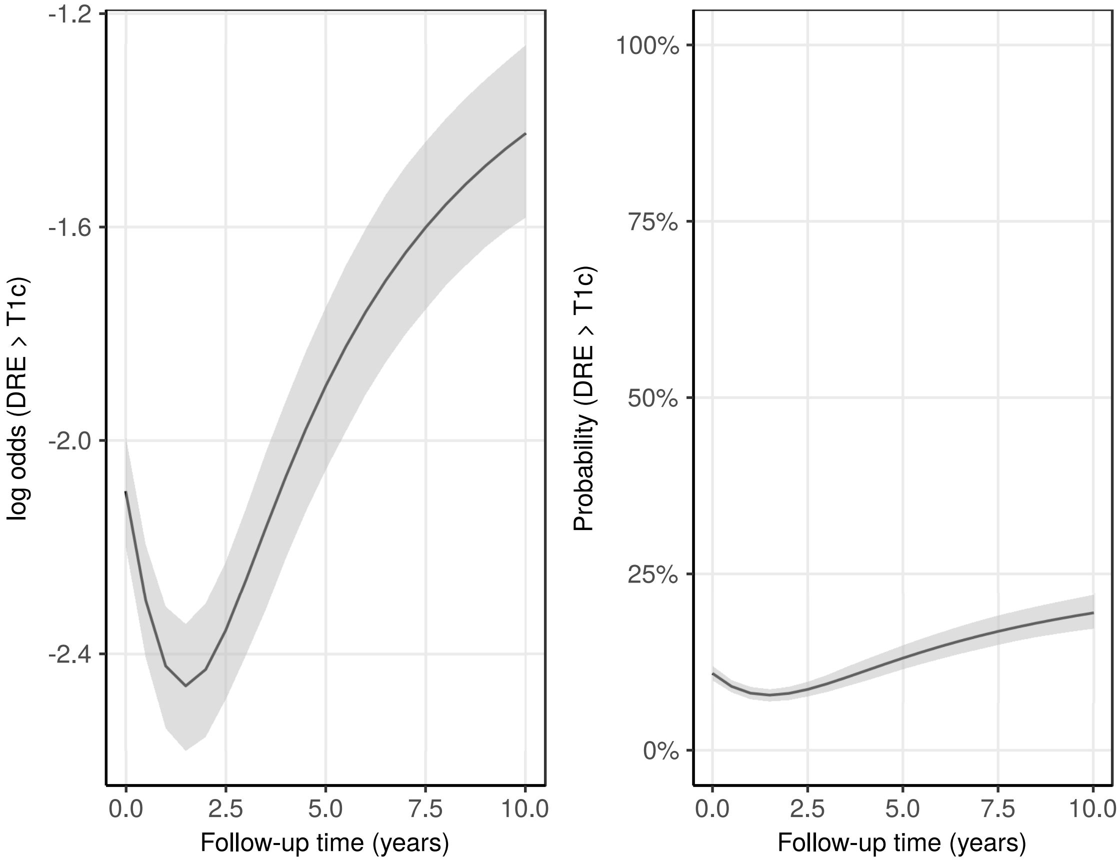


Figure 3: Fitted marginal evolution of the log odds of obtaining a DRE larger than T1c, and the corresponding marginal probability, with 95% credible interval. These results are for a hypothetical AS patient who is included in AS at the age of 70 years.

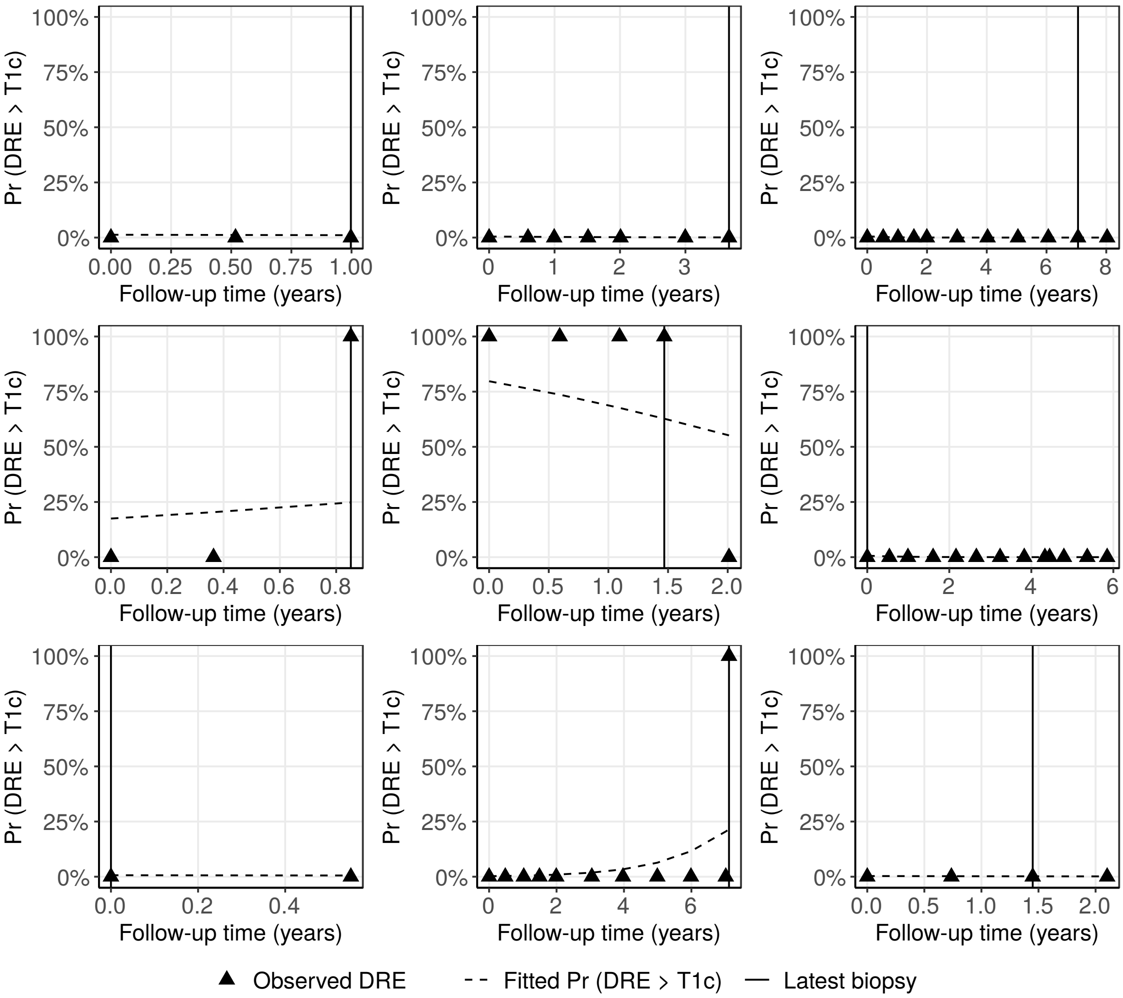


Figure 4: Observed DRE versus fitted probabilities of obtaining a DRE measurement larger than T1c, for nine randomly selected PRIAS patients. The fitted profiles utilize information from the observed DRE measurements, PSA measurements, and time of the latest biopsy. Observed DRE measurements plotted against 0% probability are equal to T1c. Observed DRE measurements plotted against 100% probability are larger than T1c.

For the PSA mixed effects sub-model parameter estimates (see Equation 2), in Table 4 we can see that the age of the patient trivially affects the baseline $\log_2(\text{PSA}+1)$ measurement. Since the longitudinal evolution of $\log_2(\text{PSA}+1)$ measurements is modeled with non-linear terms, the interpretation of the coefficients corresponding to time is not straightforward. In lieu of the interpretation, in Figure 5 we present the fitted marginal evolution of $\log_2(\text{PSA}+1)$ over a period of 10 years for a hypothetical patient who is included in AS at the age of 70 years. In addition, we present plots of observed versus fitted PSA profiles for nine randomly selected patients in Figure 6.

Table 4: Estimated mean and 95% credible interval for the parameters of the longitudinal sub-model (see Equation 2) for the PSA outcome.

| Variable | Mean | Std. Dev | 2.5% | 97.5% | P |
|---|---|---|---|---|---|
| (Intercept) | 2.701 | 0.008 | 2.686 | 2.716 | <0.001 |
| (Age − 70) | 0.003 | 0.001 | 0.001 | 0.005 | <0.001 |
| $(\text{Age} - 70)^2$ | $-4.7 \times 10^{-4}$ | $9.8 \times 10^{-5}$ | $-6.6 \times 10^{-4}$ | $-2.7 \times 10^{-4}$ | <0.001 |
| Spline: [0.00, 0.10] years | 0.054 | 0.009 | 0.037 | 0.073 | <0.001 |
| Spline: [0.10, 0.70] years | 0.177 | 0.012 | 0.151 | 0.200 | <0.001 |
| Spline: [0.70, 4.00] years | 0.194 | 0.016 | 0.161 | 0.225 | <0.001 |
| Spline: [4.00, 5.42] years | 0.341 | 0.015 | 0.312 | 0.371 | <0.001 |
| $\sigma$ | 0.137 | 0.001 | 0.135 | 0.138 | |

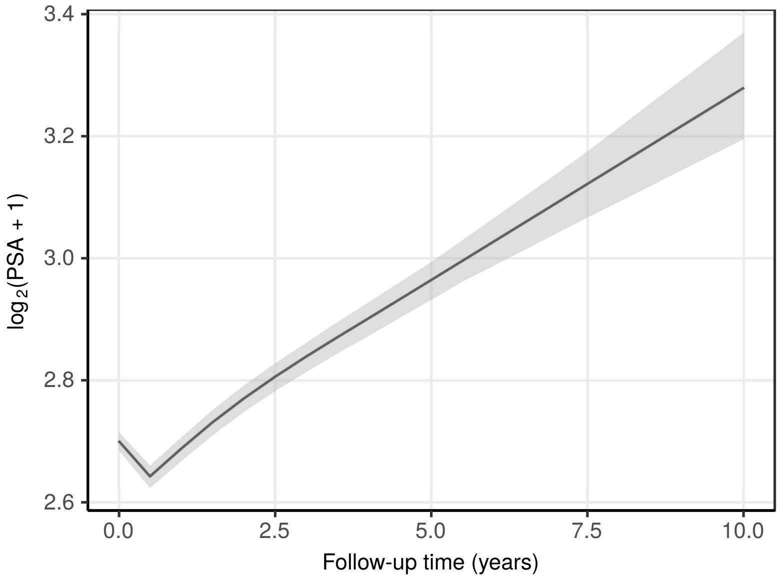


Figure 5: Fitted marginal evolution of $\log_2(\text{PSA}+1)$ measurements over a period of 10 years with 95% credible interval, for a hypothetical patient who is included in AS at the age of 70 years.

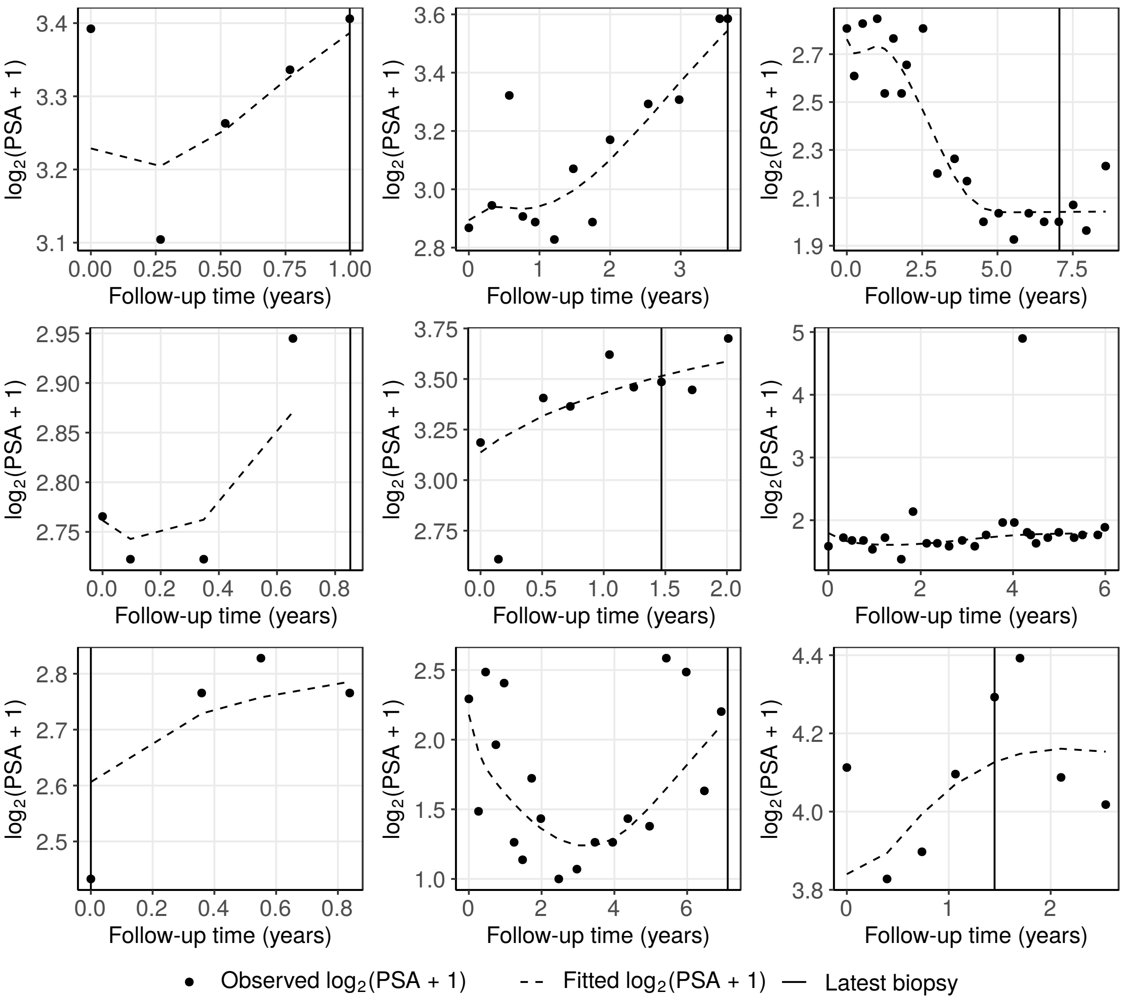


Figure 6: Fitted versus observed $\log_2(\text{PSA} + 1)$ profiles for nine randomly selected PRIAS patients. The fitted profiles utilize information from the observed PSA measurements, DRE measurements, and time of the latest biopsy.

For the relative risk sub-model (see Equation 3), the parameter estimates in Table 5 show that both $\log_2(\mathrm{PSA}+1)$ velocity, and the log odds of having DRE > T1c were significantly associated with the hazard of cancer progression.

Table 5: Estimated mean and 95% credible interval for the parameters of the relative risk sub-model (see Equation 3) of the joint model fitted to the PRIAS dataset.

| Variable | Mean | Std. Dev | 2.5% | 97.5% | P |
|---|---|---|---|---|---|
| $(\mathrm{Age}-70)$ | 0.012 | 0.006 | 0.000 | 0.022 | 0.045 |
| $(\mathrm{Age}-70)^2$ | -0.001 | 0.001 | -0.002 | 0.000 | 0.095 |
| $\mathrm{logit}\big\{\Pr(\mathrm{DRE} > \mathrm{T1c})\big\}$ | 0.147 | 0.017 | 0.115 | 0.183 | <0.001 |
| Fitted $\log_2(\mathrm{PSA}+1)$ value | 0.104 | 0.078 | -0.044 | 0.256 | 0.193 |
| Fitted $\log_2(\mathrm{PSA}+1)$ velocity | 3.396 | 0.564 | 2.376 | 4.475 | <0.001 |

It is important to note that since age, $\log_2(\mathrm{PSA}+1)$ value and velocity, and log odds of DRE > T1c are all measured on different scales, a comparison between the corresponding parameter estimates is not easy. To this end, in Table 6, we present the hazard (of cancer progression) ratio, for an increase in the aforementioned variables from their first to the third quartile. For example, an increase in log odds of DRE > T1c, from -6.650 to -4.356 (fitted first and third quartiles) corresponds to a hazard ratio of 1.402. The interpretation for the rest is similar.

Table 6: Hazard (of cancer progression) ratio and 95% credible interval (CI), for an increase in the variables of relative risk sub-model, from their first quartile ($Q_1$) to their third quartile ($Q_3$). Except for age, quartiles for all other variables are based on their fitted values obtained from the joint model fitted to the PRIAS dataset.

| Variable | $Q_1$ | $Q_3$ | Hazard ratio [95% CI] |
|---|---|---|---|
| Age | 65 | 75 | 1.129 [1.002, 1.251] |
| $\mathrm{logit}\big\{\Pr(\mathrm{DRE} > \mathrm{T1c})\big\}$ | -6.650 | -4.356 | 1.402 [1.301, 1.521] |
| $\log_2(\mathrm{PSA}+1)$ value | 2.336 | 3.053 | 1.079 [0.969, 1.201] |
| $\log_2(\mathrm{PSA}+1)$ velocity | -0.032 | 0.161 | 1.938 [1.582, 2.372] |

## Appendix B.1 Assumption of t-distributed (df=3) Error Terms

With regards to the choice of the distribution for the error term $\varepsilon_p$ for the PSA measurements (see Equation 2), we attempted fitting multiple joint models differing in error distribution, namely t-distribution with three, and four degrees of freedom, and a normal distribution for the error term. However, the model assumption for the error term were best met by the model with t-distribution having three degrees of freedom. The quantile-quantile plot of subject-specific residuals for the corresponding model in Panel A of Figure 7, shows that the assumption of t-distributed (df=3) errors is reasonably met by the fitted model.

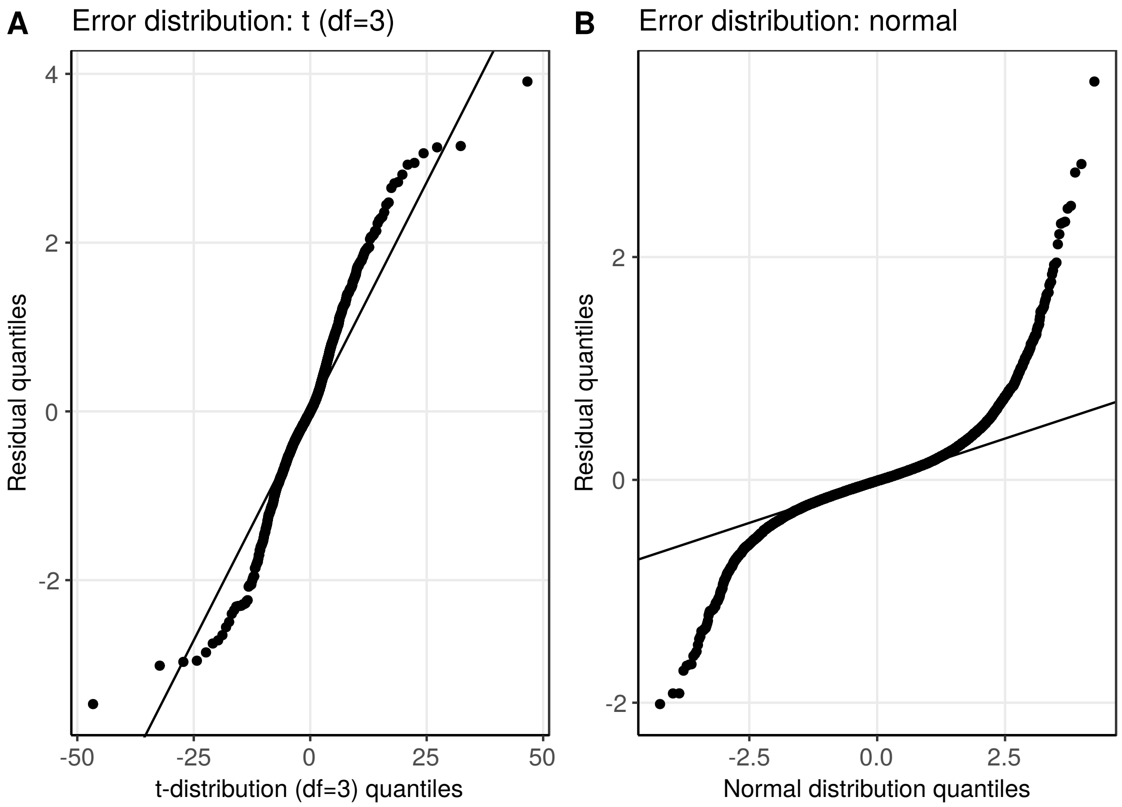


Figure 7: Quantile-quantile plot of subject-specific residuals from the joint models fitted to the PRIAS dataset. **Panel A**: model assuming a t-distribution (df=3) for the error term $\varepsilon_p$. **Panel B**: model assuming a normal distribution for the error term $\varepsilon_p$.

## Appendix B.2 Predictive Performance of the Joint Model Fitted to the PRIAS dataset

We evaluate the predictive performance of our model using two measures: the area under the receiver operating characteristic curve (AUC), and the prediction error. Given the longitudinal nature of the data at hand, in a joint model time dependent AUC and prediction errors are more relevant. More specifically, given the time of latest biopsy $t$, and history of DRE and PSA measurements up to time $s$, we are interested in a medically relevant time frame $(t, s]$, within which the occurrence of cancer progression is of interest. In the case of prostate cancer, at any point in time it is of interest to identify patients who may have obtained cancer progression in the last one year ($s - t = 1$). Using data of the patients from the PRIAS study, we calculate the AUC and prediction error (see Rizopoulos, Molenberghs, and Lesaffre, (2017) for estimation) at the following time points ($s$): year one, year two, year three, year four, and year five (95-percentile of observed cancer progression times) of follow-up in AS. The resulting AUC, and prediction error are presented in Table 7.

Table 7: Area under the receiver operating characteristic curves (AUC), and prediction error, with 95% confidence interval in brackets.

| Follow-up year | AUC | Prediction Error |
|---:|---:|---:|
| 1 | 0.651 [0.633, 0.663] | 0.055 [0.052, 0.059] |
| 2 | 0.621 [0.610, 0.640] | 0.144 [0.140, 0.148] |
| 3 | 0.748 [0.728, 0.770] | 0.076 [0.075, 0.078] |
| 4 | 0.710 [0.691, 0.736] | 0.076 [0.072, 0.079] |
| 5 | 0.592 [0.577, 0.614] | 0.107 [0.103, 0.112] |

# Appendix C Full Results of the Simulation Study

In the simulation study, we evaluate the following in-practice fixed/heuristic approaches (Inoue et al., 2018; Loeb et al., 2014) for biopsies: biopsy every year, biopsy every one and a half years, biopsy every two years and biopsy every three years. For the personalized biopsy approach we evaluate three fixed risk thresholds: 5%, 10% and 15%, and a risk threshold chosen using $F_1$ score. Lastly, we also evaluate the PRIAS schedule of biopsies. We compare all the aforementioned schedules on two criteria, namely the number of biopsies they schedule and the corresponding delay in detection of cancer progression, in years (time of positive biopsy - true time of cancer progression). The corresponding results, using $500 \times 250$ test patients are presented in Table 8.

Table 8: **Simulation study results for all patients**: Estimated first, second (median), and third quartiles for number of biopsies ($Q_1^{nb}$, $Q_2^{nb}$, $Q_3^{nb}$) and for the delay in detection of cancer progression ($Q_1^{delay}$, $Q_2^{delay}$, $Q_3^{delay}$), in years, for various biopsy schedules. The delay is equal to the difference between the time of the positive biopsy and the unobserved true time of progression. The results in the table are obtained from test patients of our simulation study.

| In-practice schedules | $Q_1^{nb}$ | $Q_2^{nb}$ | $Q_3^{nb}$ | $Q_1^{delay}$ | $Q_2^{delay}$ | $Q_3^{delay}$ |
|---|---|---|---|---|---|---|
| Every year (annual) | 3 | 10 | 10 | 0.3 | 0.5 | 0.8 |
| Every 1.5 years | 2 | 7 | 7 | 0.4 | 0.7 | 1.1 |
| Every 2 years | 2 | 5 | 5 | 0.6 | 1.1 | 1.5 |
| Every 3 years | 1 | 4 | 4 | 1.1 | 1.8 | 2.3 |
| PRIAS | 2 | 4 | 6 | 0.3 | 0.7 | 1.0 |
| Personalized approach | | | | | | |
| Risk threshold: 5% | 2 | 6 | 8 | 0.3 | 0.6 | 0.9 |
| Risk threshold: 10% | 2 | 4 | 5 | 0.3 | 0.7 | 1.0 |
| Risk threshold: 15% | 2 | 3 | 4 | 0.4 | 0.8 | 1.4 |
| Risk using $F_1$ score | 1 | 2 | 3 | 0.5 | 0.9 | 2.2 |

Since patients have varying cancer progression speeds, the impact of each schedule also varies with it. In order to highlight these differences, we divide results for three types of patients, as per their time of cancer progression. They are *fast, intermediate,* and *slow progressing* patients. Although such a division may be imperfect and can only be done retrospectively in a simulation setting, we show results for these three groups for the purpose of illustration. Roughly 50% of the patients did not obtain cancer progression in the ten year follow-up period of the simulation study. We assume these patients to be *slow progressing* patients. We assume *fast progressing* patients are the ones with an initially misdiagnosed state of cancer (Cooperberg et al., 2011) or high-risk patients who choose AS instead of immediate treatment upon diagnosis. These are roughly 30% of the population, having a cancer progression time less than 3.5 years. We label the remaining 20% patients as *intermediate progressing* patients. Table 9, Table 10, and Table 11 show the results for the *fast, intermediate,* and *slow progressing* patients, respectively.

Table 9: **Simulation study results for *fast progressing* patients (30% of all patients)**: Estimated first, second (median), and third quartiles for number of biopsies ($Q_1^{nb}$, $Q_2^{nb}$, $Q_3^{nb}$) and for the delay in detection of cancer progression ($Q_1^{delay}$, $Q_2^{delay}$, $Q_3^{delay}$), in years, for various biopsy schedules. The delay is equal to the difference between the time of the positive biopsy and the unobserved true time of progression. The results in the table are obtained from the *fast progressing* test patients of our simulation study.

| In-practice schedules | $Q_1^{nb}$ | $Q_2^{nb}$ | $Q_3^{nb}$ | $Q_1^{delay}$ | $Q_2^{delay}$ | $Q_3^{delay}$ |
|---|---|---|---|---|---|---|
| Every year (annual) | 1 | 2 | 2 | 0.3 | 0.6 | 0.9 |
| Every 1.5 years | 1 | 1 | 2 | 0.4 | 0.8 | 1.2 |
| Every 2 years | 1 | 1 | 1 | 0.7 | 1.1 | 1.5 |
| Every 3 years | 1 | 1 | 1 | 1.5 | 2.0 | 2.5 |
| PRIAS | 1 | 2 | 2 | 0.3 | 0.7 | 1.0 |
| Personalized approach | | | | | | |
| Risk threshold: 5% | 1 | 2 | 2 | 0.3 | 0.6 | 0.9 |
| Risk threshold: 10% | 1 | 1 | 2 | 0.3 | 0.7 | 1.0 |
| Risk threshold: 15% | 1 | 1 | 2 | 0.4 | 0.8 | 1.2 |
| Risk using $F_1$ score | 1 | 1 | 2 | 0.5 | 0.9 | 2.0 |

Table 10: **Simulation study results for *intermediate progressing* patients (20% of all patients)**: Estimated first, second (median), and third quartiles for number of biopsies ($Q_1^{nb}$, $Q_2^{nb}$, $Q_3^{nb}$) and for the delay in detection of cancer progression ($Q_1^{delay}$, $Q_2^{delay}$, $Q_3^{delay}$), in years, for various biopsy schedules. The delay is equal to the difference between the time of the positive biopsy and the unobserved true time of progression. The results in the table are obtained from the *intermediate progressing* test patients of our simulation study.

| In-practice schedules | $Q_1^{nb}$ | $Q_2^{nb}$ | $Q_3^{nb}$ | $Q_1^{delay}$ | $Q_2^{delay}$ | $Q_3^{delay}$ |
|---|---|---|---|---|---|---|
| Every year (annual) | 5 | 7 | 8 | 0.2 | 0.5 | 0.7 |
| Every 1.5 years | 4 | 5 | 6 | 0.3 | 0.7 | 1.0 |
| Every 2 years | 3 | 4 | 4 | 0.4 | 1.0 | 1.5 |
| Every 3 years | 2 | 3 | 3 | 0.6 | 1.3 | 2.0 |
| PRIAS | 3 | 5 | 6 | 0.3 | 0.7 | 1.3 |
| Personalized approach | | | | | | |
| Risk threshold: 5% | 5 | 6 | 7 | 0.3 | 0.6 | 0.9 |
| Risk threshold: 10% | 3 | 4 | 6 | 0.4 | 0.7 | 1.3 |
| Risk threshold: 15% | 3 | 3 | 5 | 0.4 | 0.8 | 1.7 |
| Risk using $F_1$ score | 2 | 3 | 5 | 0.5 | 1.0 | 2.4 |

Table 11: **Simulation study results for *slow progressing* patients (50% of all patients)**: Estimated first, second (median), and third quartiles for number of biopsies ($Q_1^{nb}$, $Q_2^{nb}$, $Q_3^{nb}$) and for the delay in detection of cancer progression ($Q_1^{delay}$, $Q_2^{delay}$, $Q_3^{delay}$), in years, for various biopsy schedules. The delay is equal to the difference between the time of the positive biopsy and the unobserved true time of progression. The results in the table are obtained from the *slow progressing* test patients of our simulation study. Since no cancer progression is observed in the ten year follow-up period for these patients, delay cannot be estimated, and hence is not reported.

| In-practice schedules | $Q_1^{nb}$ | $Q_2^{nb}$ | $Q_3^{nb}$ | $Q_1^{delay}$ | $Q_2^{delay}$ | $Q_3^{delay}$ |
|---|---|---|---|---|---|---|
| Every year (annual) | 10 | 10 | 10 | | | |
| Every 1.5 years | 7 | 7 | 7 | | | |
| Every 2 years | 5 | 5 | 5 | | | |
| Every 3 years | 4 | 4 | 4 | | | |
| PRIAS | 4 | 6 | 8 | | | |
| Personalized approach | | | | | | |
| Risk threshold: 5% | 6 | 7 | 9 | | | |
| Risk threshold: 10% | 4 | 4 | 6 | | | |
| Risk threshold: 15% | 2 | 3 | 4 | | | |
| Risk using $F_1$ score | 2 | 2 | 4 | | | |

# Appendix D Source Code

The R code for fitting the joint model to the PRIAS dataset, and for the simulation study are available at https://github.com/anirudhtomer/prias/tree/master/src/decision_analytic. We refer to this location as 'DATA_HOME' in the rest of this document.

## Appendix D.1 Fitting the joint model to the PRIAS dataset

**Accessing the dataset:** The PRIAS dataset is not openly accessible. However, access to the database can be requested via the contact links at www.prias-project.org.

**Formatting the dataset:** This dataset however is in the so-called wide format and also requires removal of incorrect entries. This can be done via the R script DATA_HOME/fittingModel/dataset_cleaning.R. This will lead to two R objects, namely 'prias.id' and 'prias_long'. The 'prias.id' object contains information about time of cancer progression for PRIAS patients. The 'prias_long' object contains longitudinal PSA, DRE measurements, time of biopsies and results of biopsies.

**Fitting the joint model:** We use a joint model for time to event and bivariate longitudinal data to model the evolution of PSA and DRE measurements over time, and to simultaneously model their association with the risk of cancer progression. The R package we use for this purpose is called **JMbayes** (https://cran.r-project.org/web/packages/JMbayes/JMbayes.pdf). The API we use, however, are currently not hosted on CRAN, and can be found here: https://github.com/drizopoulos/JMbayes. The joint model can be fitted via the script DATA_HOME/fittingModel/psa_dre_jointAnalysis.R. It takes roughly 6 hours to run on an Intel core-i5 machine with 4 cores, and 8GB of RAM.

The graphs presented in the main manuscript, and the supplementary material can be generated by the scripts DATA_HOME/fittingModel/demographs.R, and DATA_HOME/fittingModel/modelDiagnostic.R, respectively.

## Appendix D.2 Running the simulation study

The simulation study can be run by the following script: DATA_HOME/simulationStudy/controller.R. Although it depends on other files, the code should run without errors as long as the directory structure is maintained. An entire simulation study may take weeks to run. However, this can be controlled via the variable 'dataSetNums' in the script. Graphs related to simulation study results can be generated from the scripts DATA_HOME/simulationStudy/decisionMakingGraph.R and DATA_HOME/simulationStudy/produceResults.R

# References

Bokhorst, Leonard P et al. (2016). "A decade of active surveillance in the PRIAS study: an update and evaluation of the criteria used to recommend a switch to active treatment". In: *European Urology* 70.6, pp. 954–960.

Cooperberg, Matthew R et al. (2011). "Outcomes of active surveillance for men with intermediate-risk prostate cancer". In: *Journal of Clinical Oncology* 29.2, pp. 228–234.

De Boor, Carl (1978). *A practical guide to splines.* Vol. 27. Springer-Verlag New York.

Eilers, Paul HC and Brian D Marx (1996). "Flexible smoothing with B-splines and penalties". In: *Statistical Science* 11.2, pp. 89–121.

Gentleman, Robert and Charles J Geyer (1994). "Maximum likelihood for interval censored data: Consistency and computation". In: *Biometrika* 81.3, pp. 618–623.

Inoue, Lurdes YT et al. (2018). "Comparative Analysis of Biopsy Upgrading in Four Prostate Cancer Active Surveillance Cohorts". In: *Annals of internal medicine* 168.1, pp. 1–9.

Lin, Haiqun et al. (2000). "A latent class mixed model for analysing biomarker trajectories with irregularly scheduled observations". In: *Statistics in Medicine* 19.10, pp. 1303–1318.

Loeb, Stacy et al. (2014). "Heterogeneity in active surveillance protocols worldwide". In: *Reviews in urology* 16.4, pp. 202–203.

Pearson, Jay D et al. (1994). "Mixed-effects regression models for studying the natural history of prostate disease". In: *Statistics in Medicine* 13.5-7, pp. 587–601.

Rizopoulos, Dimitris (2012). *Joint Models for Longitudinal and Time-to-Event Data: With Applications in R.* CRC Press.

— (2016). "The R Package JMbayes for Fitting Joint Models for Longitudinal and Time-to-Event Data Using MCMC". In: *Journal of Statistical Software* 72.7, pp. 1–46.

Rizopoulos, Dimitris, Geert Molenberghs, and Emmanuel MEH Lesaffre (2017). "Dynamic predictions with time-dependent covariates in survival analysis using joint modeling and landmarking". In: *Biometrical Journal* 59.6, pp. 1261–1276.

Schröder, FH et al. (1992). "The TNM classification of prostate cancer". In: *The Prostate* 21.S4, pp. 129–138.

Tsiatis, Anastasios A and Marie Davidian (2004). "Joint modeling of longitudinal and time-to-event data: an overview". In: *Statistica Sinica* 14.3, pp. 809–834.

Turnbull, Bruce W (1976). "The empirical distribution function with arbitrarily grouped, censored and truncated data". In: *Journal of the Royal Statistical Society. Series B (Methodological)* 38.3, pp. 290–295.
